# Supplementary material for: Towards General Visual-Linguistic Face Forgery Detection(V2)
Source: arXiv:2502.20698 source file (2025-02-28)
Supplement: Supplementary file 2 [file ablation3.tex]

\begin{table}[!t]
    \centering
    
    \resizebox{\columnwidth}{!}{
    \begin{tabular}{c|cc|cc}
        \hline
        %\multicolumn{4}{|c|}{GCD-AVG}\\
        %\hline
        \multirow{2}*{Method} & \multicolumn{2}{c|}{Celeb-DF}&
        \multicolumn{2}{c}{DFDC-P}  \\
        \cline{2-5}
        % \cmidrule{2-5}
        & AUC& EER &AUC& EER \\
        \hline
        Coarse-Only&80.79&25.16&81.79&26.13\\
        % Fine-Only&64.29&29.29&65.99&38.13\\
        Fine-Pretrain&81.29&25.49&82.64&25.76\\
        Fine-and-Fine&82.19&24.43&82.95&25.53\\
        Coarse-and-Fine&\textbf{84.80}&\textbf{22.73}&\textbf{84.74}&\textbf{23.43}\\
        \hline
    \end{tabular}
    }
    \vspace{-2pt}
    \caption{Ablation of the different training strategy.}
    \label{table:ab3}
\end{table}
