# Supplementary material for: Towards General Visual-Linguistic Face Forgery Detection(V2)
Source: arXiv:2502.20698 source file (2025-02-28)
Supplement: Supplementary file 3 [file ablation4.tex]

\begin{table}[!t]
    \centering
    
    \resizebox{0.9\columnwidth}{!}{
    \begin{tabular}{c|cc|cc}
        \hline
        %\multicolumn{4}{|c|}{GCD-AVG}\\
        %\hline
        \multirow{2}*{Method} & \multicolumn{2}{c|}{Celeb-DF}&
        \multicolumn{2}{c}{DFDC-P}  \\
        \cline{2-5}
        % \cmidrule{2-5}
        & AUC& EER &AUC& EER \\
        \hline
        % Prompt1&77.21&29.55&77.39&30.36\\
        CoOp   &82.50&24.60&81.66&26.57\\
        \hline
        Prompt 1&82.17&25.18&79.19&26.13\\
        Prompt 2&81.60&26.78&82.04&26.26\\
        Prompt 3&83.32&24.40&83.09&24.90\\
        \hline
        Prompt 4&\textbf{84.80}&\textbf{22.73}&\textbf{84.74}&\textbf{23.43}\\
        \hline
    \end{tabular}
    }
    \vspace{-2pt}
    \caption{Ablation of different coarse-grained prompts.}
    \label{table:ab4}
\end{table}
