# Supplementary material for: Towards General Visual-Linguistic Face Forgery Detection(V2)
Source: arXiv:2502.20698 source file (2025-02-28)
Supplement: Supplementary file 5 [file alg_test.tex]

\begin{algorithm}[!h]
    
    \caption{Testing period}
    \begin{algorithmic}[1]%显示行号
        \Require{Coarse-grained label set C, Fine-grained prompt set P, image encoder $E_i$, text encoder $E_t$, input image $x$.}
        \State  $l_C=E_t(C)$ 
        \State  $l_F=E_t(P)$ 
        \State  $v_x=E_i(x)$
        \State $coarse\_result,\_ = argmax(s(v_x,l_C)$
        \State Use $coarse\_result$ calculate AUC and EER
        \If {Need fine-grained result}
            \State $fine\_result,index = argmax(s(v_x,l_F)$
            \State \textbf{Return} coarse\_result, AUC, EER, P[index]
        \Else
            \State \textbf{Return} coarse\_result, AUC, EER
        \EndIf
    \end{algorithmic}
    \label{alg:test}
    
\end{algorithm}
